# Supplementary material for: Pic2Word: Mapping Pictures to Words for Zero-shot Composed Image Retrieval
Source: arXiv:2302.03084 source file (2023-05-15)
Supplement: Supplementary file 1 [file appendix.tex]

% CVPR 2023 Paper Template
% based on the CVPR template provided by Ming-Ming Cheng (https://github.com/MCG-NKU/CVPR_Template)
% modified and extended by Stefan Roth (stefan.roth@NOSPAMtu-darmstadt.de)

\documentclass[10pt,twocolumn,letterpaper]{article}

%%%%%%%%% PAPER TYPE  - PLEASE UPDATE FOR FINAL VERSION
%\usepackage[review]{cvpr}      % To produce the REVIEW version
\usepackage{cvpr}              % To produce the CAMERA-READY version
%\usepackage[pagenumbers]{cvpr} % To force page numbers, e.g. for an arXiv version

% Include other packages here, before hyperref.
\usepackage{graphicx}
\usepackage{amsmath}
\usepackage{amssymb}
\usepackage{booktabs}
\usepackage{mathtools}
\usepackage{multirow}
\usepackage{array, makecell} %
\usepackage{enumitem}

\input{math_commands.tex}

\usepackage{xcolor}
\usepackage{pifont}
%

% It is strongly recommended to use hyperref, especially for the review version.
% hyperref with option pagebackref eases the reviewers' job.
% Please disable hyperref *only* if you encounter grave issues, e.g. with the
% file validation for the camera-ready version.
%
% If you comment hyperref and then uncomment it, you should delete
% ReviewTempalte.aux before re-running LaTeX.
% (Or just hit 'q' on the first LaTeX run, let it finish, and you
%  should be clear).
\usepackage[pagebackref,breaklinks,colorlinks]{hyperref}

% Support for easy cross-referencing
\usepackage[capitalize]{cleveref}
\crefname{section}{Sec.}{Secs.}
\Crefname{section}{Section}{Sections}
\Crefname{table}{Table}{Tables}
\crefname{table}{Tab.}{Tabs.}
\usepackage{caption}
\usepackage{subcaption}

%%%%%%%%% PAPER ID  - PLEASE UPDATE
 % *** Enter the CVPR Paper ID here

\begin{document}

%%%%%%%%% TITLE - PLEASE UPDATE

\title{Supplementary Material for Pic2Word}

%\author{%
%  Kuniaki Saito$^{1,2}$\thanks{Work done during internship at Google Cloud AI Research.}\:,\; Kihyuk Sohn$^{3}$\:,\; Xiang Zhang$^{2}$\:,\; Chun-Liang Li$^{2}$\:,\; \\
%  \textbf{Chen-Yu Lee$^{2}$\:,\;Kate Saenko$^{1,4}$\:,\;Tomas Pfister$^{2}$}\\
%  \texttt{\{keisaito, saenko\}@bu.edu} \\
%  \texttt{\{kihyuks,fancyzhx,chunliang,chenyulee,tpfister\}@google.com}\\[.2cm]
%  $^{1}$Boston University, $^{2}$Google Cloud AI Research, $^{3}$Google Research, $^{4}$MIT-IBM Watson AI Lab\\
%}

\iffalse
\author{First Author\\
Institution1\\
Institution1 address\\
{\tt\small firstauthor@i1.org}
% For a paper whose authors are all at the same institution,
% omit the following lines up until the closing ``}''.
% Additional authors and addresses can be added with ``\and'',
% just like the second author.
% To save space, use either the email address or home page, not both
\and
Second Author\\
Institution2\\
First line of institution2 address\\
{\tt\small secondauthor@i2.org}
}
\fi
\maketitle

\input{zero_compose/latex/paragraphs/exp_details}
\input{zero_compose/latex/paragraphs/exp_appendix}
%%%%%%%%% BODY TEXT
\vspace{-3mm}

%%%%%%%%% REFERENCES
{\small
\bibliographystyle{ieee_fullname}
\bibliography{egbib}
}

\end{document}
